# Supplementary material for: Sensor Allocation and Online-Learning-based Path Planning for Maritime Situational Awareness Enhancement: A Multi-Agent Approach
Source: arXiv:2307.02790 source file (2023-11-27)
Supplement: Supplementary file 1 [file appendix_neurips_2023.tex]

\appendix

\section*{Supplementary Material}

\section{Overview of POMDP and Nominal Belief-State Optimization (NBO)} \label{subsection:pomdp}

A POMDP comprises six different components, namely $\mathcal{X}$, $\mathcal{A}$, $\mathcal{O}$, $\mathcal{T}$, $\mathcal{Z}$ and $\Hat{\mathcal{C}}$. Here, $\mathcal{X}$ is used to represent the possible states of both mobile sensors and targets while $\mathcal{A}$ is a set of the mobile sensors' actions. In addition, $\mathcal{O}$ is a set of observations. $\mathcal{T}$ is the state-transition function that defines how the system moves from one state to another. $\mathcal{Z}$ is the observation likelihood function that relates the observations to the states and actions. Finally, $\Hat{\mathcal{C}}$ represents the cost function that specifies the benefits of each action. The objective of a POMDP is to identify a policy where the lowest expected cost is achieved. Here, the policy is determined by selecting an action at each time step.
%\subsection{Problem Formulation}
According to~\cite{Ragi2013} and~\cite{Li2022}, we have 

\begin{itemize}
    \item \underline{State}: The POMDP's state at time step $t$ defined by $\chi_t$ includes the states of cameras $\chi^{\mathcal{C}}_t$, the states of target vessels $\chi^{\mathcal{V}}_t$, and the states of filter $\mathcal{F}_t$ $(\chi_t=(\chi^{\mathcal{C}}_t,\chi^{\mathcal{V}}_t,\mathcal{F}_t))$. Here, only the camera states and the filter states are fully observable. In particular, the filter states $\mathcal{F}_t$ contain tracks of $|\mathcal{V}|$ targets; and it is represented by Gaussian distribution with mean $\xi_t=\xi_{t|t}$ and covariance $\bold{\text{P}}_t=\bold{\text{P}}_{t|t}$ $(\mathcal{F}_t=(\xi_t,\bold{\text{P}}_t))$.
    
    \item \underline{Actions}: The cameras' action at time step $t$ defined by $a_t$ consists speeds and moving angles of $|\mathcal{C}|$ cameras \textcolor{blue}{on the sea surface}. 
    Similar to~\cite{Han2020}, the movement of cameras in the maritime environment is modelled as follows:
    \begin{equation}
        \begin{aligned}
            \begin{cases}
                x^c_{t+1} = x^c_t + s^c_t \cdot \text{cos}(\phi^c_t) \cdot 
                \Delta t\\
                y^c_{t+1} = y^c_t + s^c_t \cdot \text{sin}(\phi^c_t) \cdot \Delta t
            \end{cases},            
        \end{aligned}
        \label{eq:camera_motion_model}
    \end{equation}
    where $x^c_t$ and $y^c_t$ are positions of camera $c$ in a 2-D coordinate system at time step $t$. Additionally, $s^c_t$ and $\phi^c_t$ is the speed and the moving angle of camera $c$ at time step $t$.

    \item \underline{Observations and Observation Law}: The observations of the targets' positions at time step $t$ are given by Eq.~\eqref{eq:observations}.

\item \underline{State Transition}: The camera state, first, evolves according to Eq.~\eqref{eq:camera_motion_model}. Then, the evolution of the target state is determined using Eq.~\eqref{eq:target_motion_model}. Finally, the tracker state follows Kalman filter equations and joint probabilistic data association. 

    \item \underline{Cost function}: With the goal that is to minimize the mean-squared error (MSE) between the estimated and true positions of targets, the cost function is given by:
    \begin{equation}
        \Hat{C}(\chi_t,a_t) = \mathbb{E}\left[\lVert \chi^{\mathcal{V}}_{t+1} - \xi_{t+1} \rVert ^2|\chi_t,a_t\right],
    \end{equation}
    where $\mathbb{E}[\dots|\chi_t,a_t]$ is the conditional expectation if action $a_t$ is performed in state $\chi_t$ at time step $t$.
    
    \item \underline{Belief state}: The belief state at time step $t$ is given by $b_t=(b^{\mathcal{C}}_t,b^{\mathcal{V}}_t,b^{\xi}_t,b^{\bold{\text{P}}}_t)$ where $b^{\mathcal{C}}_t=\delta(\chi^{\mathcal{C}}-\chi^{\mathcal{C}}_t)$, $b^{\xi}_t=\delta(\xi-\xi_t)$ and $b^{\bold{\text{P}}}_t=\delta(\bold{\text{P}}-\bold{\text{P}}_t)$. In addition, $b^{\mathcal{V}}_t$ is the posterior distribution of target belief state. 
\end{itemize}
Consequently, we write the objective function over a time horizon $H$ in the belief states as follows:
\begin{equation}
    J_H(b_0) = \mathbb{E}\left[\sum_{t=0}^{H-1} \Hat{c}(\chi_t,a_t)|b_0\right],
    \label{eq:objective_function}
\end{equation}
where $\Hat{c}(\chi_t,a_t) = \int \Hat{C}(\chi,a_t) \cdot b_t(\chi) d\chi$. According to the optimality of Bellman's principle, we determine the optimal policy at time step $t=0$ as follows: $\pi_0^\star(b_0) = \argmin_{a} \{\Hat{c}(b_0,a) + \mathbb{E}[J^\star_{H-1}(b_1)|b_0,a]\}$
where $a$ is an action, $J^\star_{H-1}(b_1)$ is the optimal cumulative cost within $H-1$ time steps, and $J^\star_{H-1}(b_1) = \min_a\{ \Hat{c}(b_1,a) + \mathbb{E}[J^\star_{H-2}(b_2)|b_1,a] \}$. Therefore, the optimal policy at time step $t$ is expressed as:
\begin{equation}
\pi_t^\star(b_t) = \argmin_{a} \{\Hat{c}(b_t,a) + \mathbb{E}[J^\star_{H-1-t}(b_{t+1})|b_t,a]\}. 
\label{eq:policy}
\end{equation}

Due to the complexity of calculating $\mathbb{E}[J^\star_{H-1-t}(b_{t+1})|b_t,a]$ in Eq.~\eqref{eq:policy}, we employ an approximation approach, Nominal Belief-State Optimization (NBO). Specifically, the objective function in Eq.~\eqref{eq:objective_function} is approximated as 
\begin{equation}
J_H(b_0) \approx \sum_{t=0}^{H-1} \Tilde{c}(\Tilde{b}_t,a_t),
\label{eq:new-objective_function}
\end{equation}
where $\Tilde{b}_t$ is the nominal belief state at time step $t$. To calculate the nominal belief states of a target $v \in \mathcal{V}$ $(\Tilde{b}^{\mathcal{V}_v}_{t+1},\dots,\Tilde{b}^{\mathcal{V}_v}_{H-t-1})$, we employ the target's track $\Tilde{\xi}^v_{t}$ and $\Tilde{\bold{P}}^v_{t}$ which are obtained using Kalman filter method and joint probabilistic data association. Then, we have $\Tilde{b}^{\mathcal{V}_v}_t \sim N(\Tilde{\xi}^v_t;\Tilde{\bold{P}}^v_t)$ and $\Tilde{\xi}^v_{t+1}=\bold{F}_v \cdot \Tilde{\xi}^v_{t}$. Additionally, $\Tilde{\bold{P}}^v_{t+1}$ is computed as follows~\cite{Ragi2013}:
\begin{equation}
    \Tilde{\bold{P}}^v_{t+1}=
    \begin{cases}
        \frac{1}{\frac{1}{\Tilde{\bold{P}}^v_{t+1|t}}+\bold{S}^v_{t+1}} & \text{if $v$ is observed},\\
        \Tilde{\bold{P}}^v_{t+1|t} & \text{otherwise} 
    \end{cases}.
\end{equation}
Since target $v$ can be tracked by radar $r$, AIS and camera $c \in \mathcal{C}$, we have $\Tilde{\xi}^{rv}_{t+1}=\bold{F}_v \cdot \Tilde{\xi}^{rv}_{t}$, $\Tilde{\xi}^{\text{AIS}v}_{t+1}=\bold{F}_v \cdot \Tilde{\xi}^{\text{AIS}v}_{t}$ and $\Tilde{\xi}^{cv}_{t+1}=\bold{F}_v \cdot \Tilde{\xi}^{cv}_{t} \label{eq:estimation}$, and
\begin{equation}
\begin{aligned}
    &\Tilde{\bold{P}}^{rv}_{t+1}=
    \begin{cases}
        \frac{1}{\frac{1}{\Tilde{\bold{P}}^{rv}_{t+1|t}}+\bold{S}^{rv}_{t+1}} & \text{if $v$ is observed by $r$},\\
        \Tilde{\text{P}}^{rv}_{t+1|t} & \text{otherwise} 
    \end{cases}\\
    &\Tilde{\bold{P}}^{\text{AIS}v}_{t+1}=
    \begin{cases}
        \frac{1}{\frac{1}{\Tilde{\bold{P}}^{\text{AIS}v}_{t+1|t}}+\bold{S}^{\text{AIS}v}_{t+1}} & \text{if $v$ is observed by AIS},\\
        \Tilde{\bold{P}}^{\text{AIS}v}_{t+1|t} & \text{otherwise} 
    \end{cases}\\
    &\Tilde{\bold{P}}^{cv}_{t+1}=
    \begin{cases}
        \frac{1}{\frac{1}{\Tilde{\bold{P}}^{cv}_{t+1|t}}+\bold{S}^{cv}_{t+1}} & \text{if $v$ is observed by $c$},\\
        \Tilde{\bold{P}}^{cv}_{t+1|t} & \text{otherwise} 
    \end{cases},
\end{aligned}
\end{equation}
where $\Tilde{\bold{P}}^{rv}_{t+1|t}=\bold{F}_v \cdot \Tilde{\bold{P}}^{rv}_{t} \cdot \bold{F}^T_v + \bold{Q}^v_t$, $\Tilde{\bold{P}}^{\text{AIS}v}_{t+1|t}=\bold{F}_v \cdot \Tilde{\bold{P}}^{\text{AIS}v}_{t} \cdot \bold{F}^T_v + \bold{Q}^v_t$ and $\Tilde{\bold{P}}^{cv}_{t+1|t}=\bold{F}_v \cdot \Tilde{\bold{P}}^{cv}_{t} \cdot \bold{F}^T_v + \bold{Q}^v_t$. Additionally, $\bold{S}^{rv}_{t+1}={\bold{H}^r_{t+1}}^T \cdot \bold{R}^{rv}_{t+1} \cdot \bold{H}^r_{t+1}$, $\bold{S}^{\text{AIS}v}_{t+1}={\bold{H}^{\text{AIS}}_{t+1}}^T \cdot \bold{R}^{\text{AIS}}_{t+1} \cdot \bold{H}^{\text{AIS}}_{t+1}$ and $\bold{S}^{cv}_{t+1}={\bold{H}^c_{t+1}}^T \cdot \bold{R}^{cv}_{t+1} \cdot \bold{H}^c_{t+1}$. We assume that measurements would be available at time step $t+1$ if the nominal mean position of target $v$ at time step $t+1$, i.e., $\Tilde{\xi}^{rv}_{t+1}$, $\Tilde{\xi}^{\text{AIS}v}_{t+1}$ and $\Tilde{\xi}^{cv}_{t+1}$, are in the coverage area of radar $r$ and AIS, and the FOV of camera $c$, respectively. As a result, the cost function in Eq.~\eqref{eq:new-objective_function} is rewritten as $\Tilde{c}(\Tilde{b}_t,a_t) = \sum_{v\in \mathcal{V}} \text{Tr} \left(\Tilde{\bold{P}}^v_{t+1}\right)$ with $\Tilde{\bold{P}}^v_{t+1}=\frac{1}{\frac{1}{\Tilde{\bold{P}}^{rv}_{t+1}}+\frac{1}{\Tilde{\bold{P}}^{\text{AIS}v}_{t+1}}+\frac{1}{\Tilde{\bold{P}}^{cv}_{t+1}}}$.

\newpage

\section{Psuedo-code of the Proposed Sensor Allocation and RML-based Distributed Path Planning Approach}  \label{alg:RML}
\begin{algorithm}[h]
\scriptsize
    \caption{\textbf{The Proposed Sensor Allocation and RML-based Distributed Path Planning Approach}}
    \begin{algorithmic}[1]
        \STATE \textbf{Input:} A camera set $\mathcal{C}$, a target set $\mathcal{V}$, the current position of $\mathcal{C}$ cameras, and  the information about $\mathcal{V}$ targets collected up to the current time step $t=\Tilde{t}+0$;
        \STATE \textbf{Output:} $\Hat{x}^{cv}_t,s^c_t,\phi^c_t$ ;
        \STATE \textbf{Step 0 (Initialization):}
        \STATE \quad Formulate the problem under the POMDP framework;
        \STATE \textbf{Step 1 (Multi-Sensor Allocation Algorithm):}
        \STATE \quad \textbf{for} $t=\Tilde{t}+0,\Tilde{t}+1,\dots,\Tilde{t}+H-1$
        \STATE \quad \quad \textbf{If} $t=\Tilde{t}+0$
        \STATE \quad \quad \quad Compute the matrix $\mathbf{M}_t$ using Eqs.~\eqref{eq:beta} and~\eqref{eq:matrix_m};
        \STATE \quad \quad \quad Calculate $\Hat{x}^{cv}_t$ using the $3$-step process in section~\ref{sensor allocation};
        \STATE \quad \quad \textbf{else}
        \STATE \quad \quad \quad $\Hat{x}^{cv}_t=\Hat{x}^{cv}_{t-1}$;
        \STATE \quad \quad \textbf{end}
        \STATE \quad \textbf{end for}
        \STATE \textbf{Step 2 (RML-based Distributed Multi-Agent Path Planning Algorithm):}
        %\STATE \quad Initializes each camera $c$'s action selection policy at $t=0$: $\pi^c_0(j) \leftarrow \frac{1}{|\mathcal{A}^c_0|}$ $\forall j\in \mathcal{A}^c_0$.
        \STATE \quad \textbf{for} $t=\Tilde{t}+0,\Tilde{t}+1,\dots,\Tilde{t}+H-1$
        %\STATE \quad \quad Camera $c$ plays an action $a^c_{t}=j \in \mathcal{A}^c_{t}$ from its probability distribution $\pi_{t}^c(j)$.\\
        %\STATE \quad \quad The action which camera $c$ has chosen is updated to all other cameras.\\
        \STATE \quad \quad \textbf{Regret-matching procedure} run independently by each camera $c \in \mathcal{C}$:
        \STATE \quad \quad \textbf{\{} Initialize the probability distribution at $\tau=1$ of time step $t$: $\pi^c_{t,1}(j) \leftarrow \frac{1}{|\mathcal{A}^c_{t,1}|}$ $\forall j\in \mathcal{A}^c_{t,1}$  %$\pi^c_{t,1}(j) = \pi^c_{t}(j) \quad \forall j \in \mathcal{A}^c_{t,\tau}$ 
        \STATE \quad \quad \quad \textbf{for} $\tau=1,2,\dots,T$
        \STATE \quad \quad \quad \quad \textbf{Action selection:}       
        \STATE \quad \quad \quad \quad \quad Select action $a^c_{t,\tau}=j$ from its probability distribution $\pi_{t,\tau}^c(j).$
        \STATE \quad \quad \quad \quad \quad Update to all other cameras with the action that has been chosen.\\
        \STATE \quad \quad \quad \quad \textbf{Utility update:} 
        \STATE \quad \quad \quad \quad \quad Calculates the utility $u^c_{t,\tau}(j,a^{-c}_{t,\tau})$ using Eq.~\eqref{eq:utility}.
        \STATE \quad \quad \quad \quad \textbf{for} $k\in \mathcal{A}^c_{t,\tau}\setminus\{j\}$
        \STATE \quad \quad \quad \quad \quad \textbf{Expected utilities:} 
        \STATE \quad \quad \quad \quad \quad \quad Given the decisions made by the other cameras~$-c$, calculate the expected utility $u^c_{t,\tau}(k,a^{-c}_{t,\tau})$ using Eq.~\eqref{eq:utility}.
        \STATE \quad \quad \quad \quad \quad \textbf{Regret update:} 
        \STATE \quad \quad \quad \quad \quad \quad Determine the cumulative regret $\Hat{D}^c_{t,\tau}(j,k)$ for not choosing action $k$ using Eq.~\eqref{eq:probability}.
        \STATE \quad \quad \quad \quad \quad \textbf{Strategy update:}
        \STATE \quad \quad \quad \quad \quad \quad Compute the next action probability $\pi^c_{t,\tau+1}(k)$ using Eq.~\eqref{eq:updated_probability}.
        \STATE \quad \quad \quad \quad \quad \quad Compute the probability that camera $c$ plays the same action selected in the current iteration using Eq.~\eqref{eq:rml}.
        \STATE \quad \quad \quad \quad \textbf{end for}
        \STATE \quad \quad \quad \textbf{end for}
        \STATE \quad \quad \quad Pick action $a^c_{t,T+1}=j$ according to the probability distribution $\pi^c_{t,T+1}(j)$.
        \STATE \quad \quad \quad $s^c_t=s^c_{t,T+1}$ and $\phi^c_t=\phi^c_{t,T+1}$. \textbf{\}}
        \STATE \quad \textbf{end for}
        \STATE \textbf{Step 3 (Stopping test):}
        \STATE \quad \textbf{If} all $|\mathcal{V}|$ targets are observed
        \STATE \quad \quad Stop \textbf{Algorithm~\ref{alg:RML}};
        \STATE \quad \textbf{else}
        \STATE \quad \quad Go to \textbf{Step 1};
        \STATE \quad \textbf{end}
    \end{algorithmic}
\end{algorithm}

\newpage

\section{Experimental Settings} \label{table:settings}

\begin{table}[h]
\caption{Experiment Settings.}
\begin{center}

\begin{tabular}{@{}lr@{}}\toprule
 \hline
 \textbf{Parameter} & \textbf{Value} \\ %[2ex] 
 \hline
 \multicolumn{2}{c}{\textbf{Radar}}\\
 $p^r$ & $13$ \\
 \hline
 \multicolumn{2}{c}{\textbf{Automatic identification systems (AIS)}}\\
 $\sigma^{\text{AIS}}$ & $10^3$ \\
 \hline
 \multicolumn{2}{c}{\textbf{Mobile cameras}}\\
 $p^c$ & $13$ \\
 Number of mobile cameras $|\mathcal{C}|$& $[2;10]$ \\
 HFOV of each camera $c$ & $3 \degree$ \\
 Detection range of each camera $c$ & $16$ km \\
 $\Delta t$ & $1$ s \\ 
 $H$ & $[1;5]$ time steps \\
 $\alpha_1$, $\alpha_2$, $\alpha_3$ & 1 \\
 $D_{\min}$ & $80$ m \\
 $D_{\max}$ & $16$ km \\
 $D_{\text{safe}}$ & $100$ m \\
 $s_{\min}$ & $0$ knot ($= 0$ m/s) \\
 $s_{\max}$ & $18$ knots ($\approx 9$ m/s)\\
 $\Phi_{\max}$ & $180 \degree$  \\
 $T$ & $10$ \\
 $\epsilon$ & $7 \times 10^5$ \\
 $\lambda$ & $0.5$ \\
 Number of cameras' speed levels $|\mathcal{L}_s|$ & $[2;10]$ \\
 Number of cameras' moving angle levels $|\mathcal{L}_m|$ & $[2;10]$ \\
 \hline
 \multicolumn{2}{c}{\textbf{Targets}}\\
 Number of targets $|\mathcal{V}|$ & $[5;100]$ \\
 Speed of each target $v$ & $[0;18]$ knots ($\approx [0;9]$ \text{m/s})\\
 $\sigma_v$ & $3$ \\
 \hline
\end{tabular}
\end{center}

\end{table}
